# Supplementary material for: Reversible Jump Metropolis Light Transport using Inverse Mappings
Source: arXiv:1704.06835 source file (2017-04-22)
Supplement: Supplementary file 1 [file appendix.tex]

% !TEX root=paper.tex
\appendix
\section{Computing Jacobians}

In \secref{sec:inversion-problems}, we derived \equref{eq:reversible-jump-map-probability} in terms of the Jacobians of the sampling techniques and their inverses. We will now discuss how to compute these Jacobians more concretely for entire paths and relate them to the sampling PDFs.

As seen earlier in this section, $\Pinv_i(\ubar)$ can usually be written in terms of a chain of low-dimensional sampling techniques. Analogously, Jacobians derived from $\Pinv_i$ decompose into a product,
\begin{align}
    \big\vert\JacSub{\xbar,\ubar_{\xbar}}{\Pinv_j}(\ubar)\big\vert &= \prod\limits_{l=1}^\stCount \big\vert\JacSub{\xbarAt{l},\ubar_{\xbarAt{l}}}{g_l}(\ubarAt{l})\big\vert \\
    \big\vert\JacSub{\ubar_{\auxbar},\auxbar}{\Pfor_j}(\auxbar)\big\vert^{-1} &= \prod\limits_{l=1}^\stCount \big\vert\JacSub{\ubar_{\auxbarAt{l}},\auxbarAt{l}}{g_l^{-1}}(\auxbarAt{l})\big\vert^{-1}
%    \big\vert\JacSub{\xbar,\ubar_{\xbar}}{\Pinv_j}(\vbar)\big\vert\cdot\big\vert\JacSub{\aux,\ubar_{\aux}}{\Pfor_j}(\vbar)\big\vert^{-1} &= \prod\limits_{l=1}^\stCount \big\vert\JacSub{\xbarAt{l},\ubar_{\xbarAt{l}}}{g_l}(\CurrentStatePSS^{(l)})\big\vert\cdot\big\vert\JacSub{\aux^{(l)},\ubar_{\aux^{(l)}}}{g_l^{-1}}(\aux^{(l)})\big\vert^{-1}
%    \big\vert\JacSub{\xbar}{\Pinv_i}(\CurrentStatePSS)\big\vert &= \prod\limits_{l=1}^\stCount \big\vert\JacSub{\xbar_l}{g_l}(\CurrentStatePSS^{(l)})\big\vert \\
%    \big\vert\Jac{\Pfor_i(\xbar, \cdot)}(\aux)\big\vert^{-1} &= \prod\limits_{l=1}^\stCount \big\vert\Jac{g_l^{-1}(\xbar_l, \cdot)}(\aux^{(l)})\big\vert^{-1}
\end{align}
\cWAJ{Potentially same issue here as in Eq. (17)}
If the individual $g_l$ are exactly invertible, then these Jacobians reduce to the inverse PDF of $g_l$. We've already seen that this applies to many basic sampling algorithms used in light transport simulations (in particular, those derived using the inversion method).% If there are ambiguous intervals present, then the Jacobian of the inverse will reduce to a product of constants of the form $b - a$, which can be computed easily.

However, care needs to be taken when dealing with mixtures of strategies~(Section~\ref{sec:sampling-mixtures}). To precisely reason about this problem, we rewrite the acceptance ratio in a more general form. We say that every $g_l(\ubar)$ consists of a combination of $n_l$ techniques denoted $g_{l,k}(\ubar)$, where technique $k$ is selected with probability $\TechniqueWeight_{k}$. The non-mixture case can be recovered with $n_l=1$. We now restate the acceptance ratio as
\begin{align}
	\AcceptanceP(\CurrentStateExPSS \rightarrow \NextStateExPSS) &= \frac{\misWeightPSS_j(\NextStatePSS)\ProposalDistribution(j \rightarrow i)}{\misWeightPSS_i(\CurrentStatePSS)\ProposalDistribution(i \rightarrow j)} \frac{A_i(\ubar)}{A_j(\vbar)} \\
	A_i(\ubar) &= \prod\limits_{l=1}^\stCount a_{i,l}(\ubarAt{l}) \\
	a_{i,l}(\ubar) &= T(t_l|i)\; \big\vert\JacSub{\xbar_l,\ubar_{\xbar_l}}{g_{l,t_l}}(\ubar)\big\vert\cdot\big\vert\JacSub{\aux^{(l)},\ubar_{\aux^{(l)}}}{g_{l,t_l}^{-1}}\big\vert^{-1} \punct{.} \label{eq:per-technique-terms}
\end{align}
We use $a_{i,l}(\ubar)$ to encapsulate all terms introduced by the $l$-th sample method on the random walk.

In the following, we reason about a single sample method $g_l$ and will drop the $l$ subscript for conciseness. As with the Blinn-Phong example, we use the first element of the random number vector to select one of the sampling techniques.% For ease of notation, we assume the individual $g_t$ to be exactly invertible here.

The PDF of this mixture is simply the weighted sum of the individual PDFs,
\begin{align}
    P[g](\ubar) = \sum\limits_{t=1}^n \TechniqueWeight_t P[g_t](\ubarAt{2}\ldots) \punct{,}
\end{align}
where $P[g]$ denotes the PDF of $g$. However, the Jacobians of this mixture are
\begin{align}
    \big\vert\JacSub{\xbar,\ubar_{\xbar}}{g_{t}}(\ubar)\big\vert &= P[g_t](\ubarAt{2}\ldots)^{-1} \\
    \big\vert\JacSub{\ubar_{\auxbar}, \auxbar}{g_{t}^{-1}}\big\vert^{-1} &= \TechniqueWeight_t^{-1} \punct{,}
\end{align}
where $t$ is the index of the technique that was actually used to sample the path. The factor of $\TechniqueWeight_t$ stems from the parametrization of $u_1$ in the inverse.

The factor $a_{i,l}(\ubar)$ contributed by this mapping is not its PDF, but the scaled PDF of the sub-technique that was actually used. This is unfortunate, since it no longer allows us to reason about the acceptance ratio as we did at the end of \secref{sec:rmj} and achieve an optimal acceptance ratio.
\cJN{This was the hardest part to follow so far... I wonder if there is a way to make it easier to read.}

So far, we've neglected discussion of the third term \cJN{It appears as the first term. Maybe start with something like ``We shall now discuss the discrete probability $\ProposalDistribution(t|j)$''} of $a_{i,l}(\ubar)$: The discrete probability $\ProposalDistribution(t|j)$ of selecting the $t$-th technique during inversion. We have relative freedom in designing this distribution, and we now describe a setting that retrieves the optimal acceptance ratio. Consider
\begin{align}
    \ProposalDistribution(t|i) = \frac{\TechniqueWeight_t P[g_t](\ubarAt{2}\ldots)}{\sum\limits_{s=1}^n \TechniqueWeight_s P[g_s](\ubarAt{2}\ldots)} \punct{.}
\end{align}
This simply states that during inversion, technique $t$ should be selected with probability proportional to its likelihood of generating the given path. Reinserting into \equref{eq:per-technique-terms} yields
\begin{align}
    a_{i,l}(\ubar) &= \frac{\TechniqueWeight_t P[g_{l,t}](\ubarAt{2}\ldots)}{\sum\limits_{s=1}^n \TechniqueWeight_s P[g_{l,s}](\ubarAt{2}\ldots)} P[g_{l,t}](\ubarAt{2}\ldots)^{-1} \TechniqueWeight_t^{-1} \\
    &= \frac{1}{\sum\limits_{s=1}^n \TechniqueWeight_s P[g_{l,s}](\ubarAt{2}\ldots)} \\
    &= P[g](\ubar)^{-1} \punct{.}
\end{align}
By designing an appropriate proposal distribution, we could retrieve the original sampling PDF even for sampling mixtures. Together with an appropriate distribution for $\ProposalDistribution(i \rightarrow j)$ (\secref{sec:rmj}), this allows us to achieve an optimal acceptance ratio of $1$ for reversible multiplexed jumps.
